# Supplementary material for: Convex-Concave Zero-sum Markov Stackelberg Games
Source: arXiv:2401.12437 source file (2024-01-23)
Supplement: Supplementary file 1 [file nested_stochastic_gda.tex]

\begin{algorithm}[H]

\textbf{Inputs:} $\outerset, \innerset, \obj, \constr, \outer[][][][0], \inner[][][][0], \langmult[][][0], \numiters[\outer], \numiters[\inner], \left\{\learnrate[\outer][\iter] \right\}_{\iter = 0}^{\numiters[\outer]-1}, \left\{\learnrate[\inner][\iter] \right\}_{\iter = 0}^{\numiters[\outer]-1}$ \\
\amy{the learning rates aren't used in this algo, or in any of them, i don't think}

\textbf{Outputs:}$(\outer[][][][\iter], \inner[][][][\iter], \langmult[][][\iter])_{\iter = 0}^{\numiters[\outer]-1}$ 

\begin{algorithmic}[1]

\caption{Nested Saddle-Point-Oracle Stochastic Gradient Descent / Nested Stochastic GDA
\label{alg:nested_sgda}}

\State $\inner[][][][] \gets  \inner[][][][0]$

\State $\langmult[][][] \gets  \langmult[][][0]$

\For{$\iter = 0, \hdots, \numiters[\outer] - 1$}

    \State \textbf{Saddle-Point-Oracle SGD:}
    
    \IndState Find $(\inner[][][][\iter], \langmult[][][\iter]) \in \innerset \times \R^\numconstrs$ s.t. $\constr(\outer[][][][\iter], \inner[][][][\iter])\geq \zeros$ and 
    
    \IndState $\max_{\inner[][][\prime] \in \innerset: \constr(\outer[][][][\iter], \inner[][][\prime]) \geq \zeros}\lang(\inner[][][\prime], \langmult[][][\iter]; \outer[][][][\iter]) - \min_{\langmult[][\prime] \in \R_+^\numconstrs}\lang(\inner[][][][\iter], \langmult[][\prime]; \outer[][][][\iter]) \leq \delta $
    
    \State \textbf{Stochastic GDA:}
        
        \For{$s = 0, \hdots, \numiters[\inner] - 1$}
        \hspace{1\algorithmicindent}
        
            % \State Sample $\{\obji_\numsample \}_{\numsample = 1}^\numsamples \sim \objdistrib, \{\constri\}_{\numsample = 1}^\numsamples \sim \constrdistrib$
            
            \IndState Sample $\obji \sim \objdistrib, \constri \sim \constrdistrib$
            
            \IndState $\inner[][][] \gets  \project[{\innerset}]\left[\inner[][][] + \grad[\inner] \lang[{\obji, \constri}] (\inner[][][], \langmult[][]; \outer[][][][\iter]) \right]$
            
            \IndState  $\langmult[][][] \gets  \project[\langmults]\left[\langmult[][][] -  
            % \nicefrac{1}{\numsamples} \sum_{\numsample} 
            \grad[\langmult] \lang[{\obji, \constri}] (\inner[][][][], \langmult[][][]; \outer[][][][\iter]) \right]$
        
        % \State \textbf{IISE:}
        
        % \IndState[0] $\inner[][][] \gets  \project[\{\innerset: \constr(\outer, \inner) \geq \zeros \}]\left[\inner[][][] + \grad[\inner] \lang[\obji, \constri] (\inner[][][], \langmult[][]; \outer[][][][\iter]) \right]$
        
        % \IndState[0] $\langmult[][][] \gets  \project[\R^\numconstrs_+]\left[\langmult[][][] - \grad[\langmult] \lang[\obji, \constri] (\inner[][][][\iter], \langmult[][][\iter]; \outer[][][][\iter]) \right]$
    \EndFor
    
    \IndState $\inner[][][][\iter] \gets  \project[{\{\inner \in \innerset: \constr(\outer[][][][\iter], \inner) \geq \zeros \}}] \inner[][][][]$
    
    \IndState $\langmult[][][\iter] \gets  \langmult[][][]$
    
    \State Sample $\obji \sim \objdistrib, \constri \sim \constrdistrib$
    
    % \State Sample $\{\obji_\numsample \}_{\numsample = 1}^\numsamples \sim \objdistrib[\obji], \{\constri\}_{\numsample = 1}^\numsamples \sim \constrdistrib$
    
    \State $\outer[][][][\iter + 1] \gets \project[\outerset]\left[\outer[][][][\iter] +  
    % \nicefrac{1}{\numsamples} \sum_{\numsample} 
    \grad[\outer] \lang[{\obji, \constri}] (\inner[][][][\iter], \langmult[][][\iter]; \outer[][][][\iter]) \right]$
\EndFor

\State \Return $(\outer[][][][\iter], \inner[][][][\iter], \langmult[][][\iter])_{\iter = 0}^{\numiters[\outer]-1}$ 

\end{algorithmic}
\end{algorithm}
