# Supplementary material for: Convex-Concave Zero-sum Markov Stackelberg Games
Source: arXiv:2401.12437 source file (2024-01-23)
Supplement: Supplementary file 2 [file oracle_simple.tex]

\begin{figure}
%\begin{wrapfigure}{L}{0.55\textwidth}
    %\vspace*{-0.1cm}
    %\begin{minipage}{0.55\textwidth}
\begin{algorithm}[H]

\textbf{Inputs:} $\outer[][][][0], \inner[][][][0], \langmult[][][0], \numiters[\outer], \numiters[\inner], (\learnrate[\outer][\iter])_{\iter}$ \\

\textbf{Outputs:}$(\outer[][][][\iter], \inner[][][][\iter], \langmult[][][\iter])_{\iter = 0}^{\numiters[\outer]-1}$ 

\begin{algorithmic}[1]

\caption{Saddle-Point-Oracle Stochastic Gradient Descent\label{alg:oracle_sgda}}
\For{$\iter = 0, \hdots, \numiters[\outer] - 1$}

    \State Find $(\inner[][][][\iter], \langmult[][][\iter]) \in \innerset \times \R^\numconstrs_+$ s.t. $\|(\inner[][][][\iter], \langmult[][][\iter])-(\inner[][][*](\outer[][][][\iter]), \langmult[][*](\outer[][][][\iter]) \| \leq \delta$
    
    \State Sample $\obji \sim \objdistrib, \constri \sim \constrdistrib$
    
    % \State Sample $\{\obji_\numsample \}_{\numsample = 1}^\numsamples \sim \objdistrib[\obji], \{\constri\}_{\numsample = 1}^\numsamples \sim \constrdistrib$
    
    \State $\outer[][][][\iter + 1] \! \! \gets \! \! \project[\outerset]\! \!\left[\outer[][][][\iter]\! + \!  
    % \nicefrac{1}{\numsamples} \sum_{\numsample} 
    \learnrate[\outer][\iter]\gradlangrv[\outer] (\inner[][][][\iter], \langmult[][][\iter]; \outer[][][][\iter], \obji, \constri) \right]$
\EndFor

\State \Return $(\outer[][][][\iter], \inner[][][][\iter], \langmult[][][\iter])_{\iter = 0}^{\numiters[\outer]-1}$ 
\end{algorithmic}
\end{algorithm}
    %\end{minipage}
    %\vspace*{-0.1cm}
%\end{wrapfigure}
\end{figure}
